# Supplementary material for: Measurement of statistical nuclear spin polarization in a nanoscale GaAs sample
Source: arXiv:1109.0411 source file (2011-10-23)
Supplement: Supplementary file 1 [file SupMat1.pdf]

# Measurement of statistical nuclear spin polarization in a nanoscale GaAs sample

Fei Xue, Dennis P. Weber, Phani Peddibhotla,  
and Martino Poggio

Department of Physics, University of Basel, Klingelbergstrasse 82, 4056 Basel, Switzerland  
E-mail: [Martino.Poggio@unibas.ch](mailto:Martino.Poggio@unibas.ch)

This video intends to clarify the fabrication process of attaching a GaAs sample to an ultrasensitive Si cantilever.

Pictures are SEM micrographs, if not stated differently.

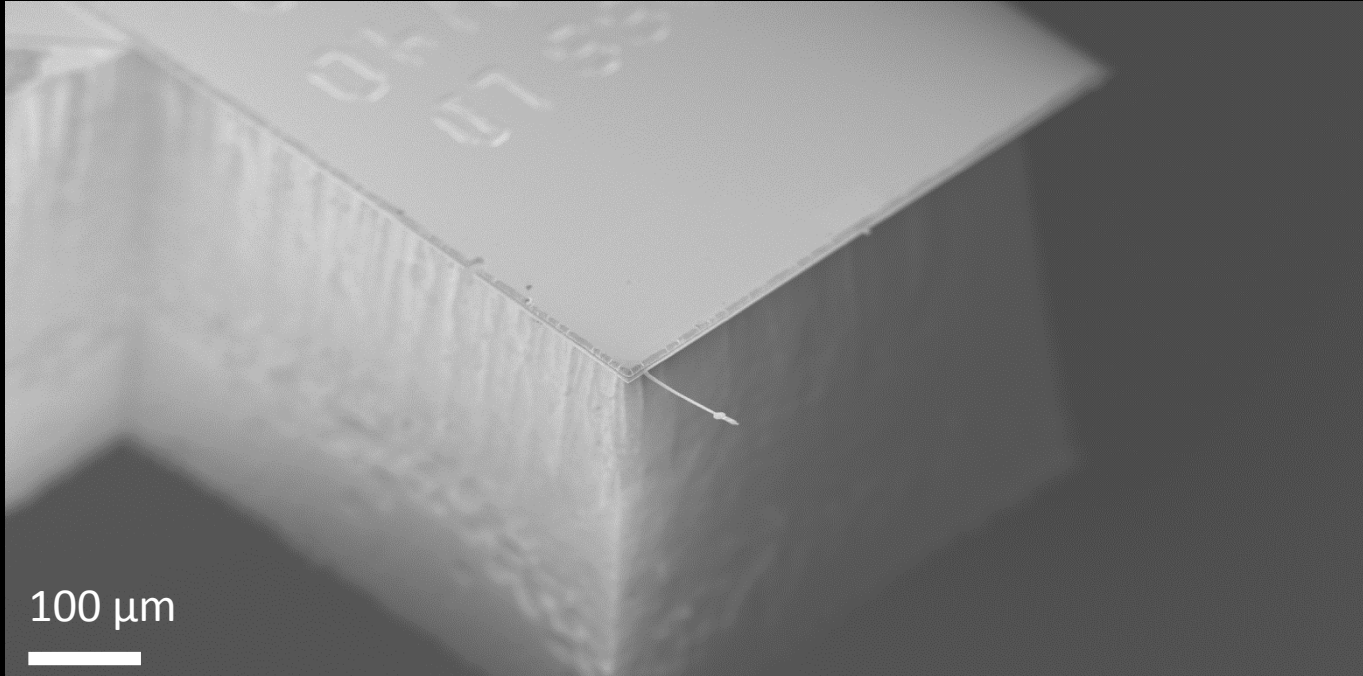

Cantilever protruding from a Si chip.

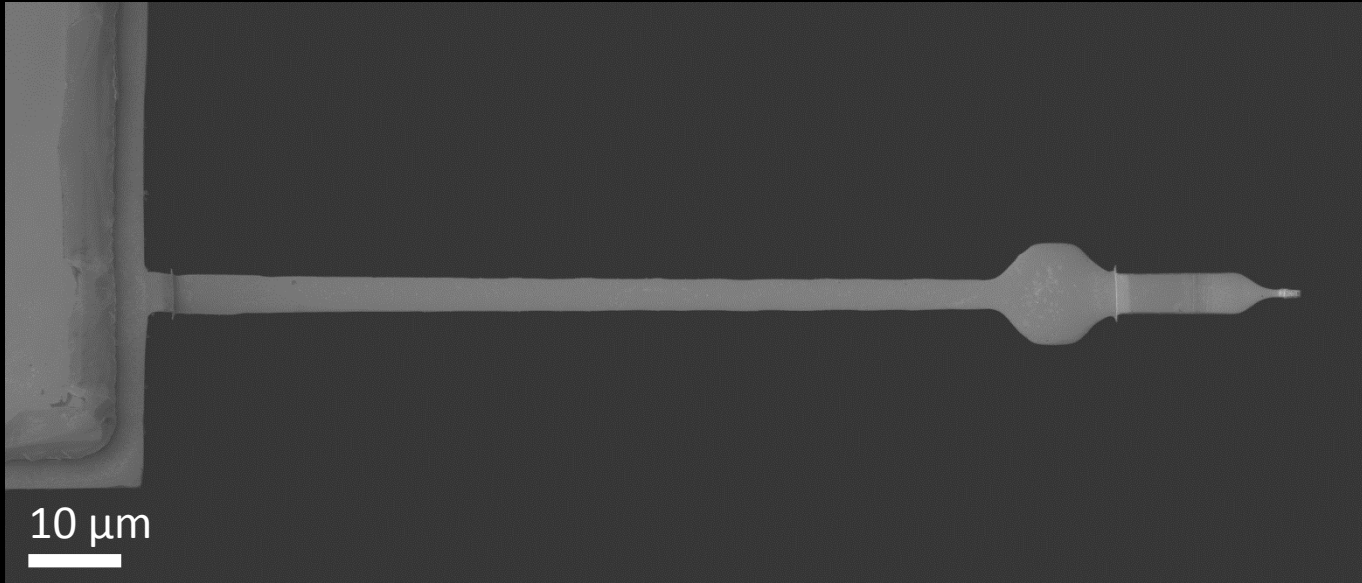

The cantilever is about 100 μm long.

# Sample preparation

The GaAs sample is affixed to the cantilever tip using a focused ion beam (FIB) technique. First, a lamella of GaAs material is cut out perpendicular to the wafer surface, and then attached to the cantilever.

This technique is also used to prepare samples for Transmission Electron Microscopy (TEM).

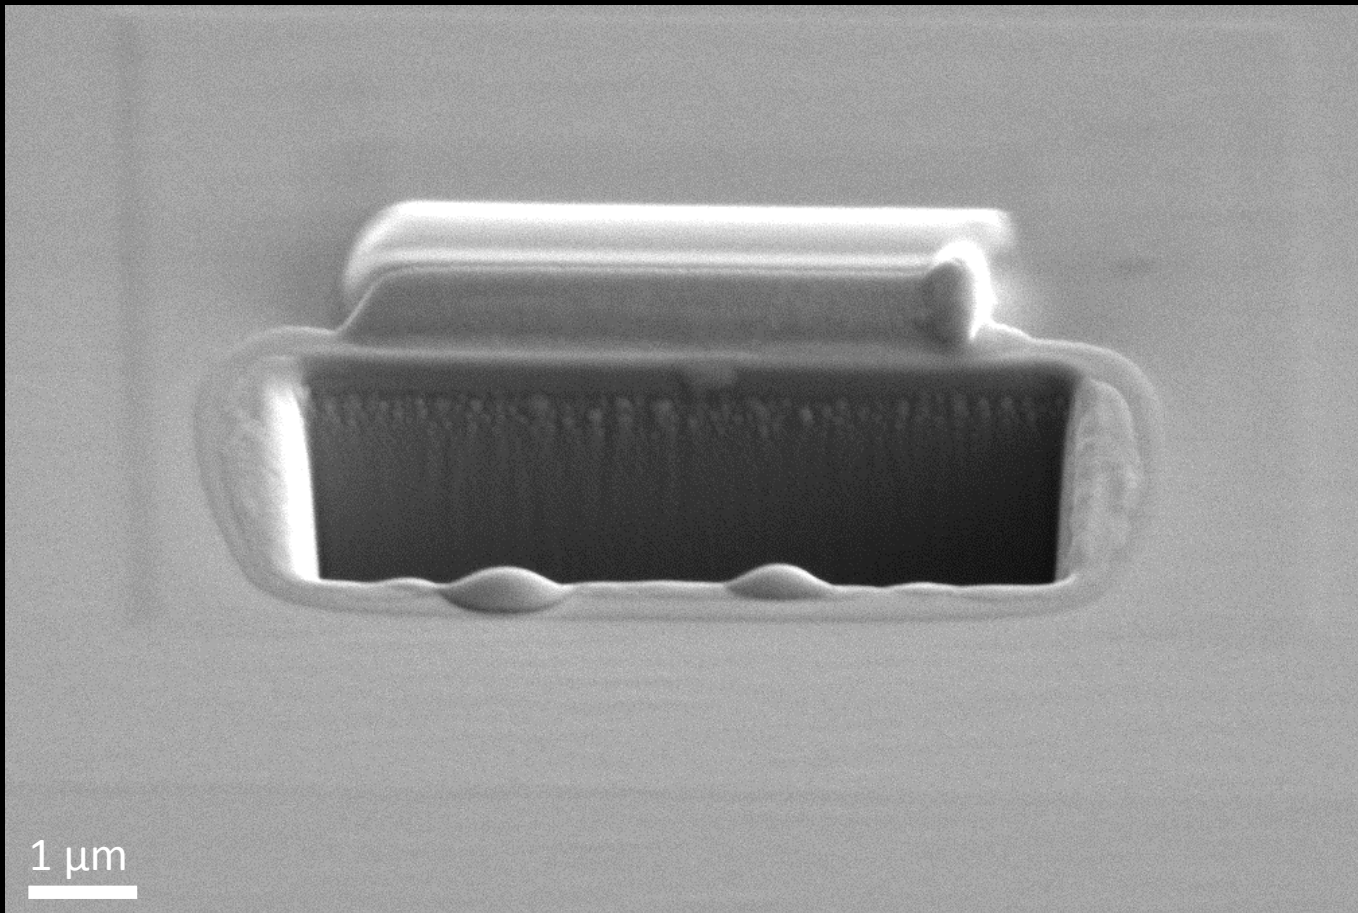

A layer of Pt (light gray) is covering the lamella to prevent damage from the FIB Ga-ions.

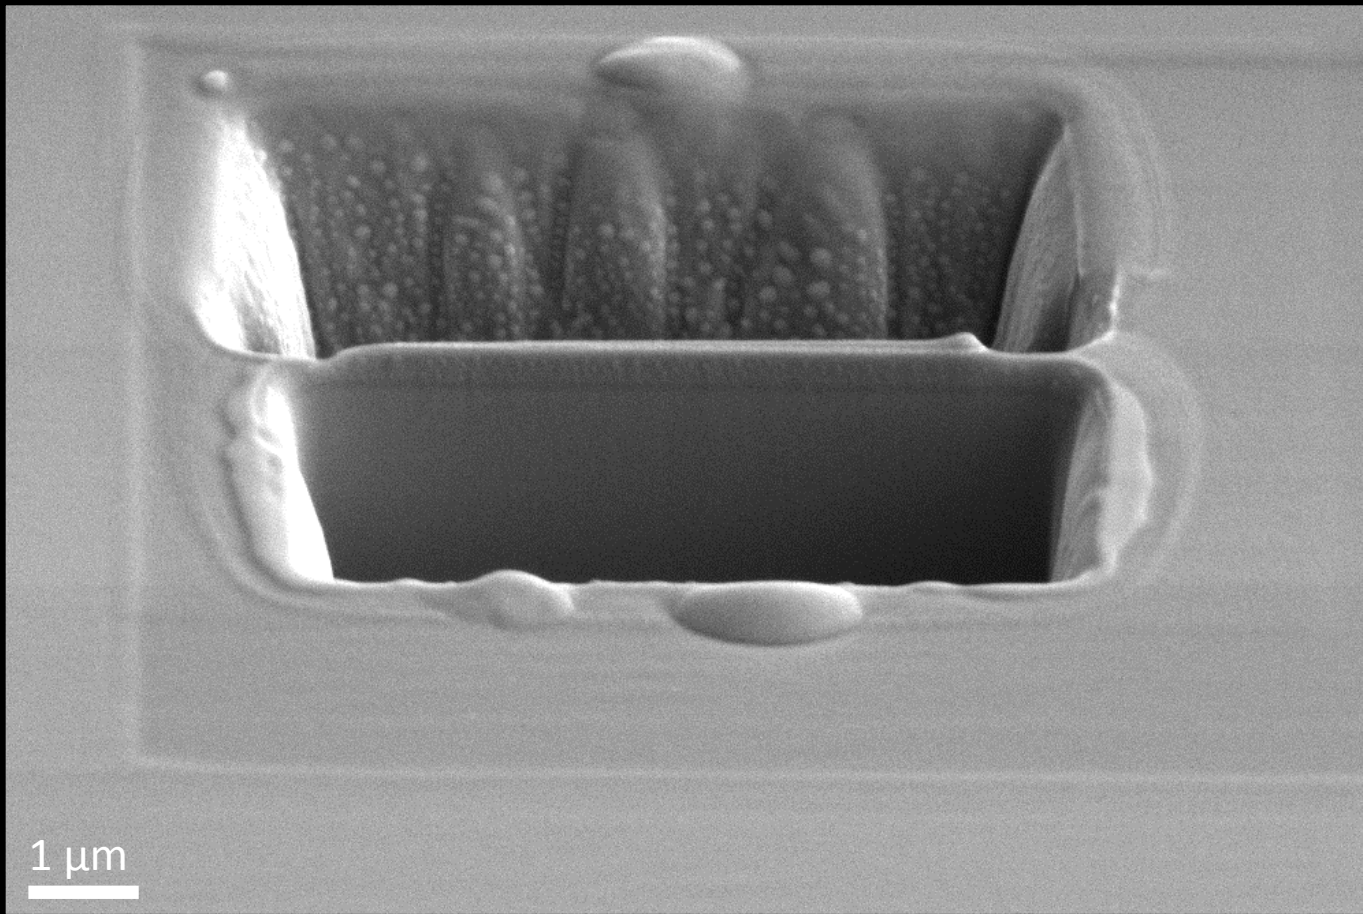

1 μm

A second groove determines the final thickness of the lamella and therefore of the GaAs sample.

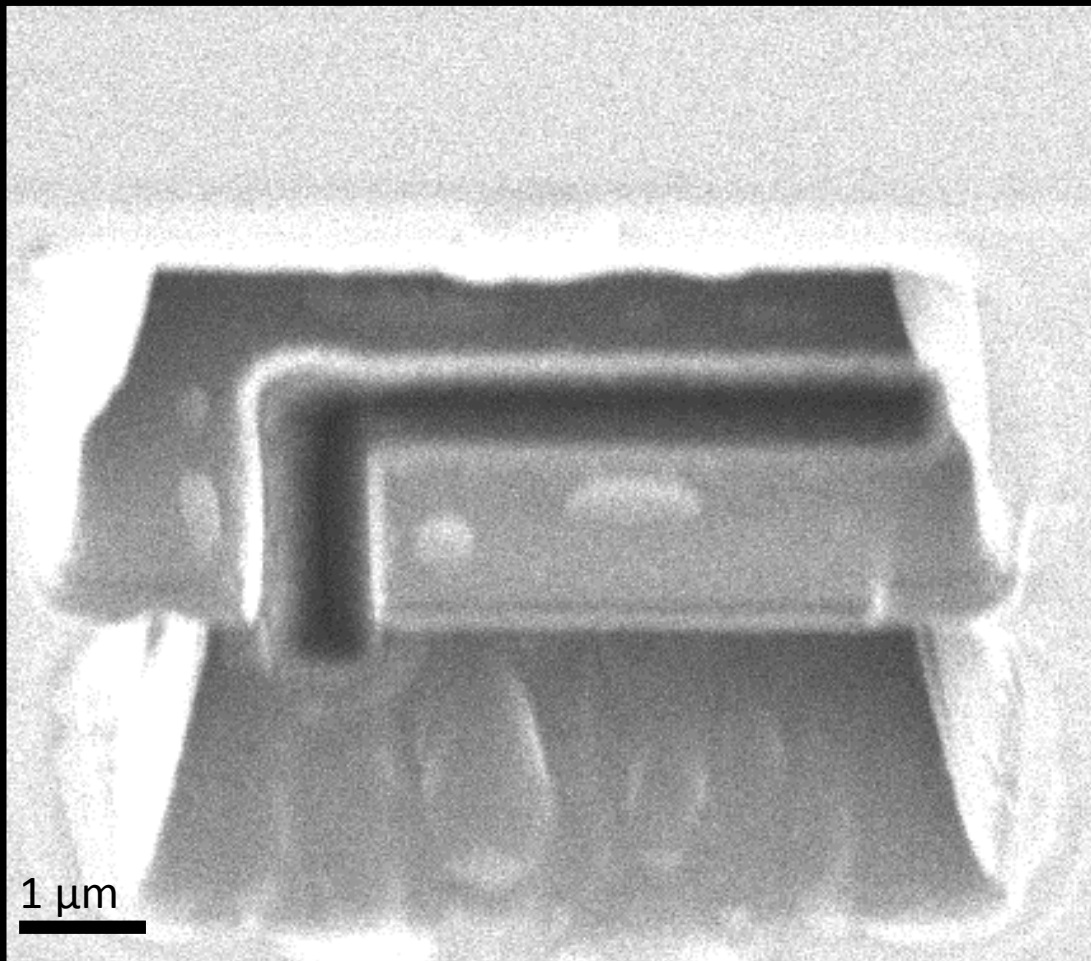

Overhead view; Ga-ion micrograph. The lamella becomes separated from the bulk material.

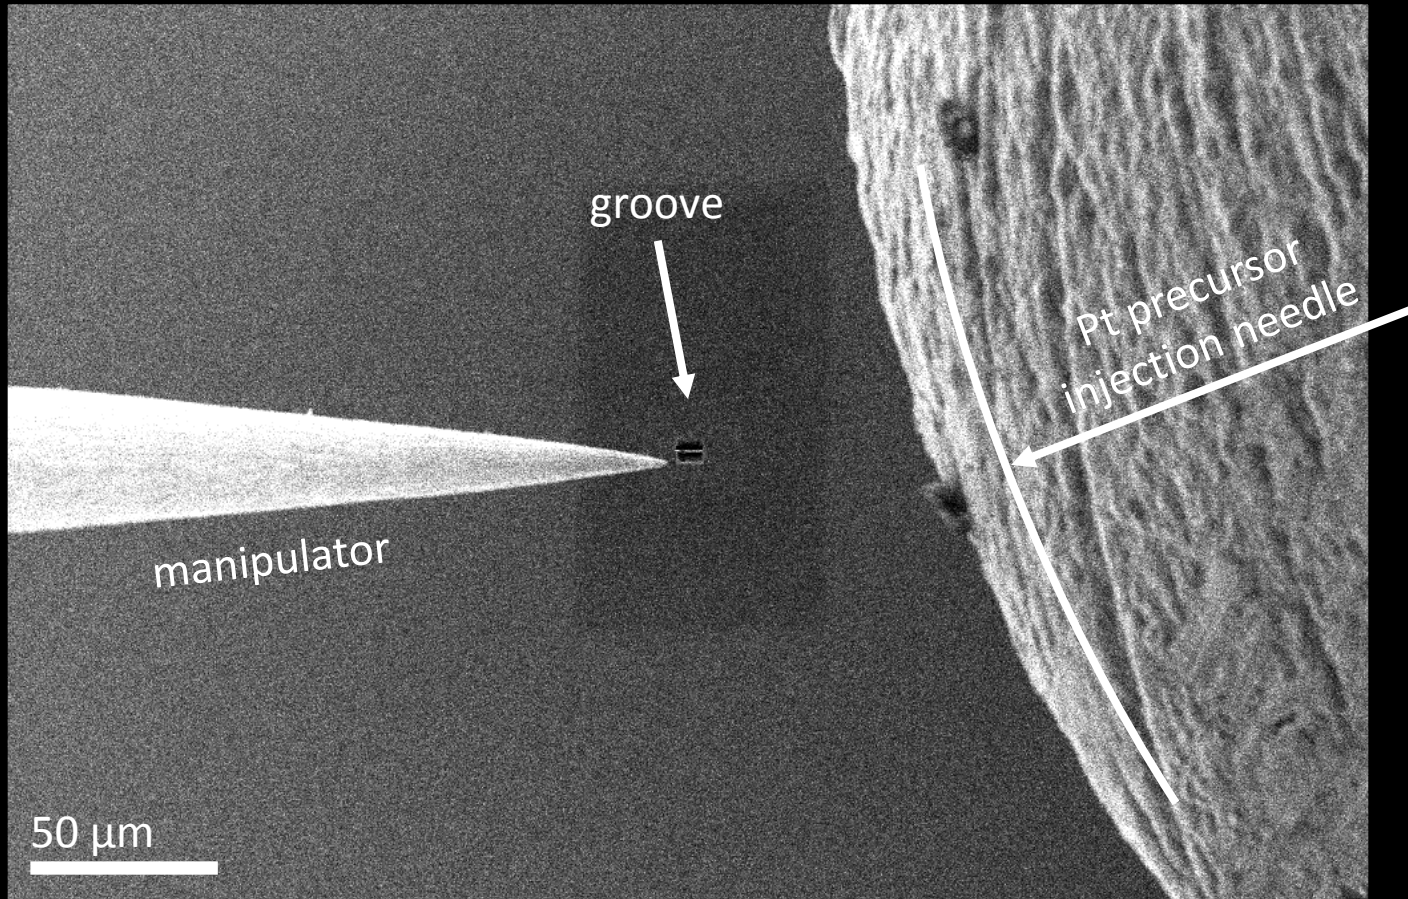

A micro-manipulator is inserted in the FIB chamber.

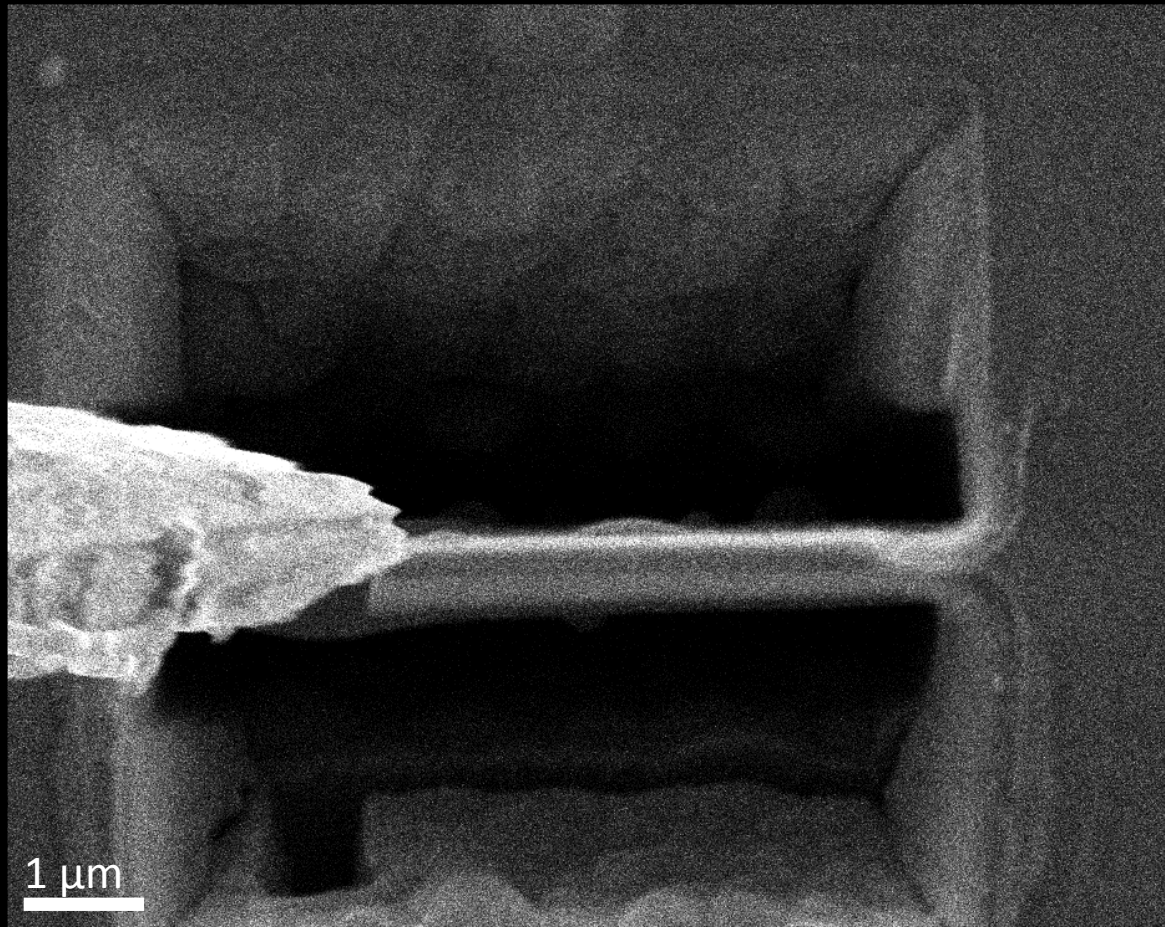

The manipulator is brought close to the lamella and Pt-welded.

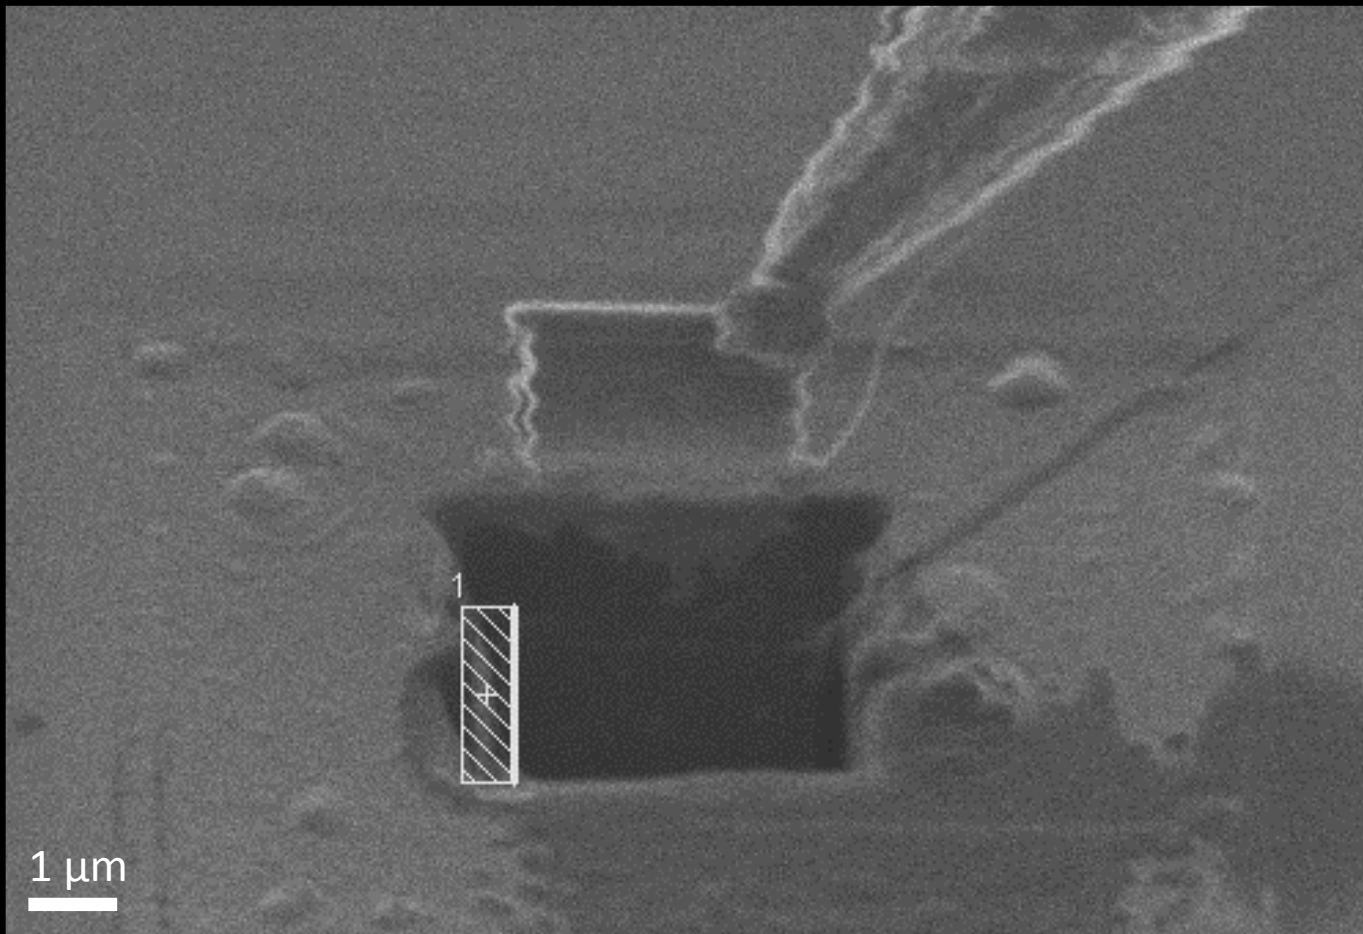

The lamella is cut off and lifted from the groove.

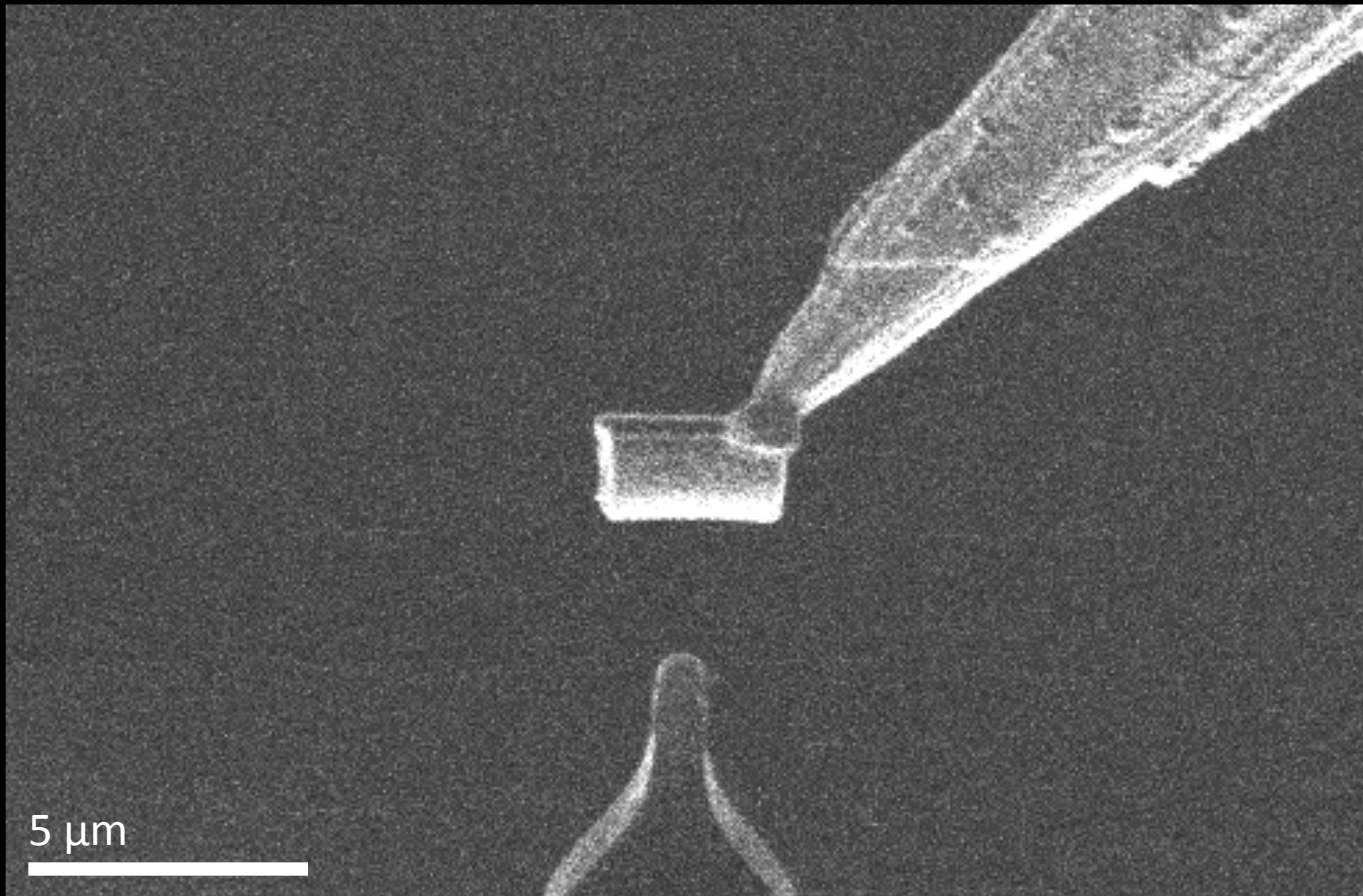

After the lamella touches the cantilever, a joint is Pt-welded.

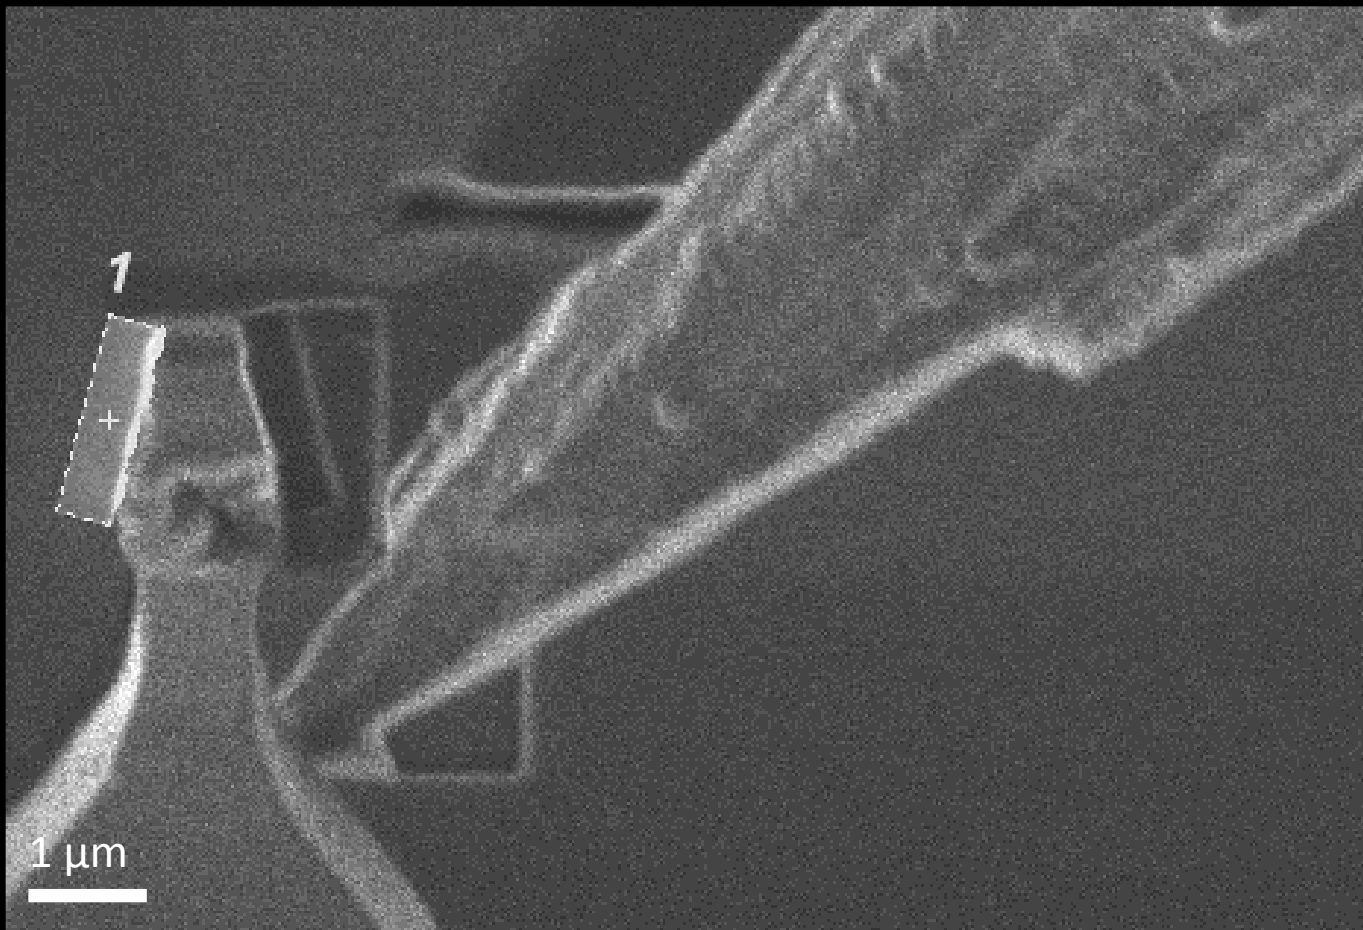

The GaAs sample is shaped to its final geometry.

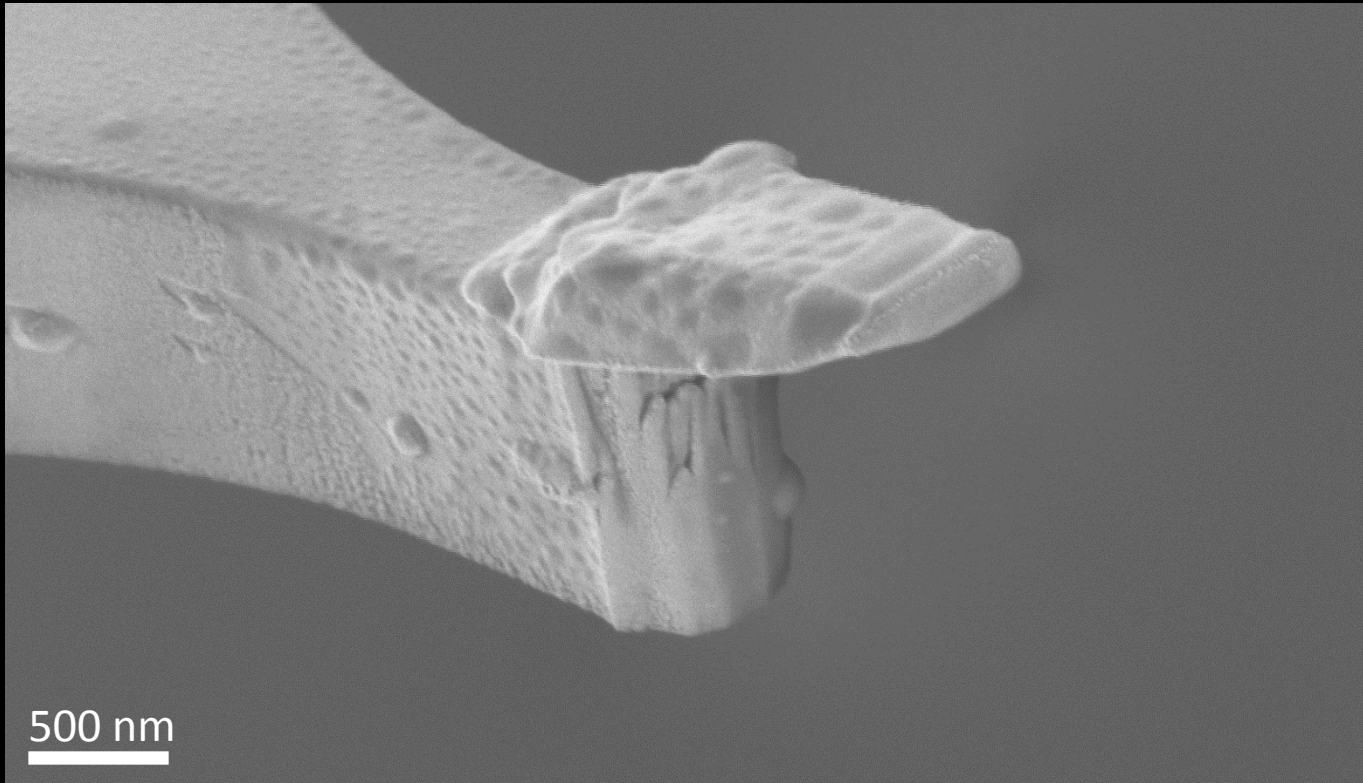

Finished GaAs sample affixed to the end of an ultrasensitive Si cantilever.

For more detailed information please refer to our letter.

The authors thank Dr. Erich Müller from the Laboratory for Electron Microscopy (LEM) at the Karlsruhe Institute of Technology (KIT) for conducting the FIB process.
